# Supplementary material for: Double excitation energies from quantum Monte Carlo using state-specific energy optimization
Source: arXiv:2207.12160 source file (2022-07-25)
Supplement: Supplementary file 2 [file supp_info.tex]

\begin{suppinfo}
Choice of input weights for the matching of multiple CIPSI wave functions; CIPSI energies, PT2 energies, and variances for the expansions used in the QMC calculations; additional QMC total and excitation energies obtained with CAS wave functions and with CIPSI determinantal components originally expressed in a CAS orbital basis.
\end{suppinfo}
