# Supplementary material for: Double excitation energies from quantum Monte Carlo using state-specific energy optimization
Source: arXiv:2207.12160 source file (2022-07-25)
Supplement: Supplementary file 5 [file cipsi-process-fig.tex]

\begin{figure}[htb]
\begin{center}
\includegraphics[scale=0.342]{cipsi-process-fig}
\caption{\label{fig:cipsi-process} Breakdown of the CIPSI calculation process. The process always begins with the MCSCF orbitals (red lines) from a CASSCF calculation (in GAMESS) which are used as the MO basis in Quantum Package. Next, for nitroxyl, glyoxal, and tetrazine, a full-CI including doubles (FCID) with zero seniority is performed. For cyclopentadienone an iterative CISD is performed up to $N_{\mathrm{det}}^{\mathrm{max}}\sim10^3$. The expansion is then truncated to between 2$-$100 determinants, depending on the system. Finally, an unrestricted CIPSI is performed up to $N_{\mathrm{det}}^{\mathrm{max}}\sim10^2-10^4$. The expansion and MCSCF orbitals are used in CHAMP for the VMC optimization and DMC calculations. Alternatively, the natural orbitals (NO) are generated and the CIPSI process is repeated (dark yellow lines). The new expansion and orbitals are then used in CHAMP.}
\end{center}
\end{figure}
