# Supplementary material for: Double excitation energies from quantum Monte Carlo using state-specific energy optimization
Source: arXiv:2207.12160 source file (2022-07-25)
Supplement: Supplementary file 6 [file cyclopentadienone-cas-table.tex]

\begin{table*}[!htb]
\caption{Summary of SA($N_{\mathrm{state}}$)-CASSCF($N_{\mathrm{e}}$, $M_{\mathrm{orb}}$) calculations on cyclopentadienone. The CASSCF energies ($E$) and excitation energies ($\Delta E$) are given in Hartree (H) and eV, respectively.}
\resizebox{\columnwidth}{!}{
\begin{tabular}{lrllllll}
\hline
% & & \multicolumn{5}{c}{MCSCF} \\
%\cline{3-7}
 & \multicolumn{1}{c}{\# CSFs} & \multicolumn{1}{c}{$E(1 ^1\mathrm{A_{1}})$} & \multicolumn{1}{c}{$E(2 ^1\mathrm{A_{1}})$} & \multicolumn{1}{c}{$E(3 ^1\mathrm{A_{1}})$} & \multicolumn{1}{c}{$\Delta E_{12}$} & \multicolumn{1}{c}{$\Delta E_{13}$} & \multicolumn{1}{c}{$\Delta E_{23}$} \\
\hline
\multicolumn{8}{l}{SA(3)} \\
\cline{1-1}
CAS(6,6)                     &   95 &  -45.749640 &  -45.519741 & -45.437557 & 6.26 & 8.49 & 2.24 \\
CAS(8,7)                     &  152 &  -45.749865 &  -45.519864 & -45.437841 & 6.26 & 8.49 & 2.23 \\
CAS(10,8)                    &  326 &  -45.752040 &  -45.521488 & -45.438852 & 6.27 & 8.52 & 2.25 \\[.5ex]
\multicolumn{8}{l}{SA(4)} \\
\cline{1-1}
CAS(6,6)                     &   95 &  -45.747679 &  -45.520726 & -45.434884 & 6.18 & 8.51 & 2.34 \\
CAS(8,7)                     &  152 &  -45.747963 &  -45.520831 & -45.435133 & 6.18 & 8.51 & 2.33 \\
CAS(10,8)                    &  326 &  -45.750131 &  -45.522663 & -45.435928 & 6.19 & 8.55 & 2.36 \\[.5ex]
\multicolumn{8}{l}{SA(5)} \\
\cline{1-1}
CAS(6,6)                     &   95 &  -45.744381 &  -45.518430 & -45.432765 & 6.15 & 8.48 & 2.33 \\
CAS(8,7)                     &  152 &  -45.747246 &  -45.518198 & -45.435403 & 6.23 & 8.49 & 2.25 \\
CAS(10,8)                    &  326 &  -45.748150 &  -45.519019 & -45.436202 & 6.23 & 8.49 & 2.25 \\
\hline
%SA(2)-CASSCF(14,10)/AVDZ$^a$ &     & -294.727767 & -294.526292 & 5.48 \\
%SA(2)-CASSCF(14,10)/AVQZ$^a$ &     & -294.803516 & -294.604540 & 5.41 \\
%\hline
%\multicolumn{5}{l}{$^a$Ref.~\citenum{loos2019}} \\
\end{tabular}
}
\label{tab:cyclopentadienone-cas}
\end{table*}
