# Supplementary material for: Double excitation energies from quantum Monte Carlo using state-specific energy optimization
Source: arXiv:2207.12160 source file (2022-07-25)
Supplement: Supplementary file 10 [file cyclopentadienone-table-SI.tex]

\begin{sidewaystable}[!htb]
\caption{Cyclopentadienone VMC and DMC results. The optimal weights ($w_1^{\mathrm{inp}}-w_2^{\mathrm{inp}}-w_3^{\mathrm{inp}}$) in the CAS basis are 0.27$-$0.35$-$0.38.}
%\caption{Cyclopentadienone VMC and DMC total energies (a.u.) and excitation energies (eV). The number of determinants (\#~det) and parameters (\#~parm) in each trial wave function are also presented. CIPSI expansions in the CAS basis use the optimized orbitals from a SA(3)-CASSCF(6,6) calculation with irrep $\mathrm{^1A_{1}}$ ($\mathrm{C_{2v}}$) using BFD pseudopotentials with the corresponding aug-cc-pVDZ basis set. The optimal weights ($w_1^{\mathrm{inp}}-w_2^{\mathrm{inp}}-w_3^{\mathrm{inp}}$) in the CAS basis are 0.27$-$0.35$-$0.38.}
\resizebox{\columnwidth}{!}{
%\rotatebox{90}{
\begin{tabular}{lrrllllllllllll}
\hline
 & & & \multicolumn{6}{c}{VMC} & \multicolumn{6}{c}{DMC} \\ 
\cline{4-9}
\cline{10-15}
\multicolumn{1}{c}{WF} & \multicolumn{1}{c}{\# det} & \multicolumn{1}{c}{\# parm} & \multicolumn{1}{c}{$E\left(1 ^1\mathrm{A_{1}}\right)$} & \multicolumn{1}{c}{$E\left(2 ^1\mathrm{A_{1}}\right)$} & \multicolumn{1}{c}{$E\left(3 ^1\mathrm{A_{1}}\right)$} & \multicolumn{1}{c}{$\Delta E_{12}$} & \multicolumn{1}{c}{$\Delta E_{13}$} & \multicolumn{1}{c}{$\Delta E_{23}$} & \multicolumn{1}{c}{$E\left(1 ^1\mathrm{A_{1}}\right)$} & \multicolumn{1}{c}{$E\left(2 ^1\mathrm{A_{1}}\right)$} & \multicolumn{1}{c}{$E\left(3 ^1\mathrm{A_{1}}\right)$} & \multicolumn{1}{c}{$\Delta E_{12}$} & \multicolumn{1}{c}{$\Delta E_{13}$} & \multicolumn{1}{c}{$\Delta E_{23}$} \\
\hline
%\multicolumn{10}{l}{State-average} \\
%\cline{1-1}
%CAS(6,6)/BFD-VDZ   && 1824 & 1139 & -46.7339(1) & -46.5129(1) & -46.4563(1)  & 6.013(4) & 7.554(4) & 0.02 & (2) & (2) & & (7) &  \\
%CIPSI-350/BDF-VDZ  &&  385 &  871 & (1) & (1) & & (4) & & 0.02 & (2) & (2) & & (8) &  \\
%\multicolumn{10}{l}{State-specific} \\
%\cline{1-1}
CAS(6,6)            &  208 &  967 & -46.7358(1) & -46.5119(1) & -46.4438(1) & 6.093(4) & 7.947(4) & 1.854(4) & -46.8322(1) & -46.6109(1) & -46.5439(1) & 6.021(6) & 7.844(6) & 1.822(6) \\[.5ex]
%CIPSI (not matched)  &  309 & 2472 & -46.7433(1) & -46.5172(1) & -46.4723(1) & 6.152(4) & 7.373(4) & (2) & (2) & (2) & (8) & (8)\\
%                     & 1550 & 4818 & -46.7531(1) & -46.5328(1) & -46.4932(1) & 5.996(4) & 7.072(4) & (2) & (2) & (2) & (7) & (7) \\
%                     & 3161 & 6066 & -46.7621(1) & -46.5403(1) & -46.5029(1) & 6.036(4) & 7.055(4) & (2) & (2) & (2) & (7) & (7) \\
\hline
\multicolumn{15}{l}{CIPSI (CAS)} \\
0.27$-$0.35$-$0.38   &  9619 & 10062 & -46.7794(2) & -46.5591(2) & -46.5220(2)  & 6.00(1) & 7.00(1) & 1.01(1) & -46.8488(2) & -46.6329(2) & -46.5967(2) & 5.87(1) & 6.86(1) & 0.99(1) \\[0.5ex]
%matching ($f$: 0.20) &  7235 &  9065 & -46.7736(2) & -46.5500(2) & -46.5185(2) & 6.08(1)  & 6.94(1) & 0.86(1) & (2) & (2) & (2) & (1) & (1) & (1) \\
matching ($f$: 0.02) &  1019 &  4735 & -46.7532(2) & -46.5281(2) & -46.4930(2) & 6.13(1) & 7.08(1) & 0.96(1) & -46.8405(2) & -46.6204(2) & -46.5854(2) & 5.99(1) & 6.94(1) & 0.95(1) \\
                     &  3036 &  6235 & -46.7663(2) & -46.5440(2) & -46.5099(2) & 6.05(1) & 6.98(1) & 0.93(1) & -46.8448(2) & -46.6278(2) & -46.5938(2) & 5.91(1) & 6.83(1) & 0.92(1) \\
                     &  7248 &  9008 & -46.7741(2) & -46.5537(2) & -46.5200(2) & 6.00(1)  & 6.91(1) & 0.92(1) & -46.8472(2) & -46.6310(2) & -46.5972(2) & 5.88(1) & 6.80(1) & 0.92(1) \\
                     & 10198 & 10557 & -46.7807(2) & -46.5605(2) & -46.5263(2) & 5.99(1)  & 6.92(1) & 0.93(1) & -46.8503(2) & -46.6330(2) & -46.5988(2) & 5.90(1) & 6.84(1) & 0.99(1) \\
\hline
\multicolumn{15}{l}{CIPSI (NO)} \\
matching ($f$: 0.02)  &  1025 &  2403 & -46.7542(2) & -46.5361(2) & -46.5000(2) & 5.94(1) & 6.92(1) & 0.98(1) & -46.8389(2) & -46.6222(2) & -46.5864(2) & 5.90(1) & 6.87(1) & 0.97(1) \\
                    &  3033 &  3645 & -46.7670(2) & -46.5485(2) & -46.5112(2) & 5.95(1) & 6.96(1) & 1.01(1) & -46.8432(2) & -46.6276(2) & -46.5908(2) & 5.87(1) & 6.87(1) & 1.00(1) \\
                    &  7151 &  5365 & -46.7826(2) & -46.5610(2) & -46.5236(2) & 6.03(1)  & 7.05(1) & 1.02(1) & -46.8480(2) & -46.6302(2) & -46.5937(2) & 5.92(1) & 6.91(1) & 0.99(1) \\
                    & 10206 &  6574 & -46.7874(2) & -46.5656(2) & -46.5292(2) & 6.04(1)  & 7.03(1) & 0.99(1) & -46.8498(2) & -46.6330(2) & -46.5965(2) & 5.90(1) & 6.89(1) & 0.99(1) \\
\hline
\multicolumn{12}{l}{TBE$^a$} & \multicolumn{1}{l}{6.00$^b$} & \multicolumn{1}{l}{6.09$^c$} & \multicolumn{1}{l}{0.09} \\
\multicolumn{12}{l}{ADC(3)/AVTZ}  & \multicolumn{1}{l}{4.59$^d$} & \multicolumn{1}{l}{6.50$^d$} & \multicolumn{1}{l}{1.91} \\
\multicolumn{12}{l}{CC2/AVTZ}     &              & \multicolumn{1}{l}{6.50$^d$} & \multicolumn{1}{l}{} \\
\multicolumn{12}{l}{CC3/AVTZ}     & \multicolumn{1}{l}{7.10$^d$} & \multicolumn{1}{l}{6.21$^d$} & \multicolumn{1}{l}{-0.89} \\
\multicolumn{12}{l}{CCSD/AVTZ}    &              & \multicolumn{1}{l}{6.68$^d$} & \multicolumn{1}{l}{} \\
\multicolumn{12}{l}{CCSDT-3/AVTZ} &              & \multicolumn{1}{l}{6.33$^d$} & \multicolumn{1}{l}{} \\
\multicolumn{12}{l}{exFCI/AVDZ}   & \multicolumn{1}{l}{5.81(39)} & \multicolumn{1}{l}{6.93(24)} & \multicolumn{1}{l}{1.10(13)} \\
\hline
\multicolumn{15}{l}{$^a$This value is `unsafe' as defined in Ref.~\citenum{questdb}.} \\
\multicolumn{15}{l}{$^b$NEVPT2/AVTZ.} \\
\multicolumn{15}{l}{$^c$CCSDT/AVDZ + ( CC3/AVTZ-CC3/AVDZ ).} \\
\multicolumn{15}{l}{$^d$Values are also `unsafe'.} \\
\end{tabular}
}%}
\label{tab:cyclopentadienone-SI}
\end{sidewaystable}
