# Supplementary material for: Double excitation energies from quantum Monte Carlo using state-specific energy optimization
Source: arXiv:2207.12160 source file (2022-07-25)
Supplement: Supplementary file 14 [file glyoxal-overlap-fig.tex]

\begin{figure}[htb]
\begin{center}
\includegraphics[scale=0.4]{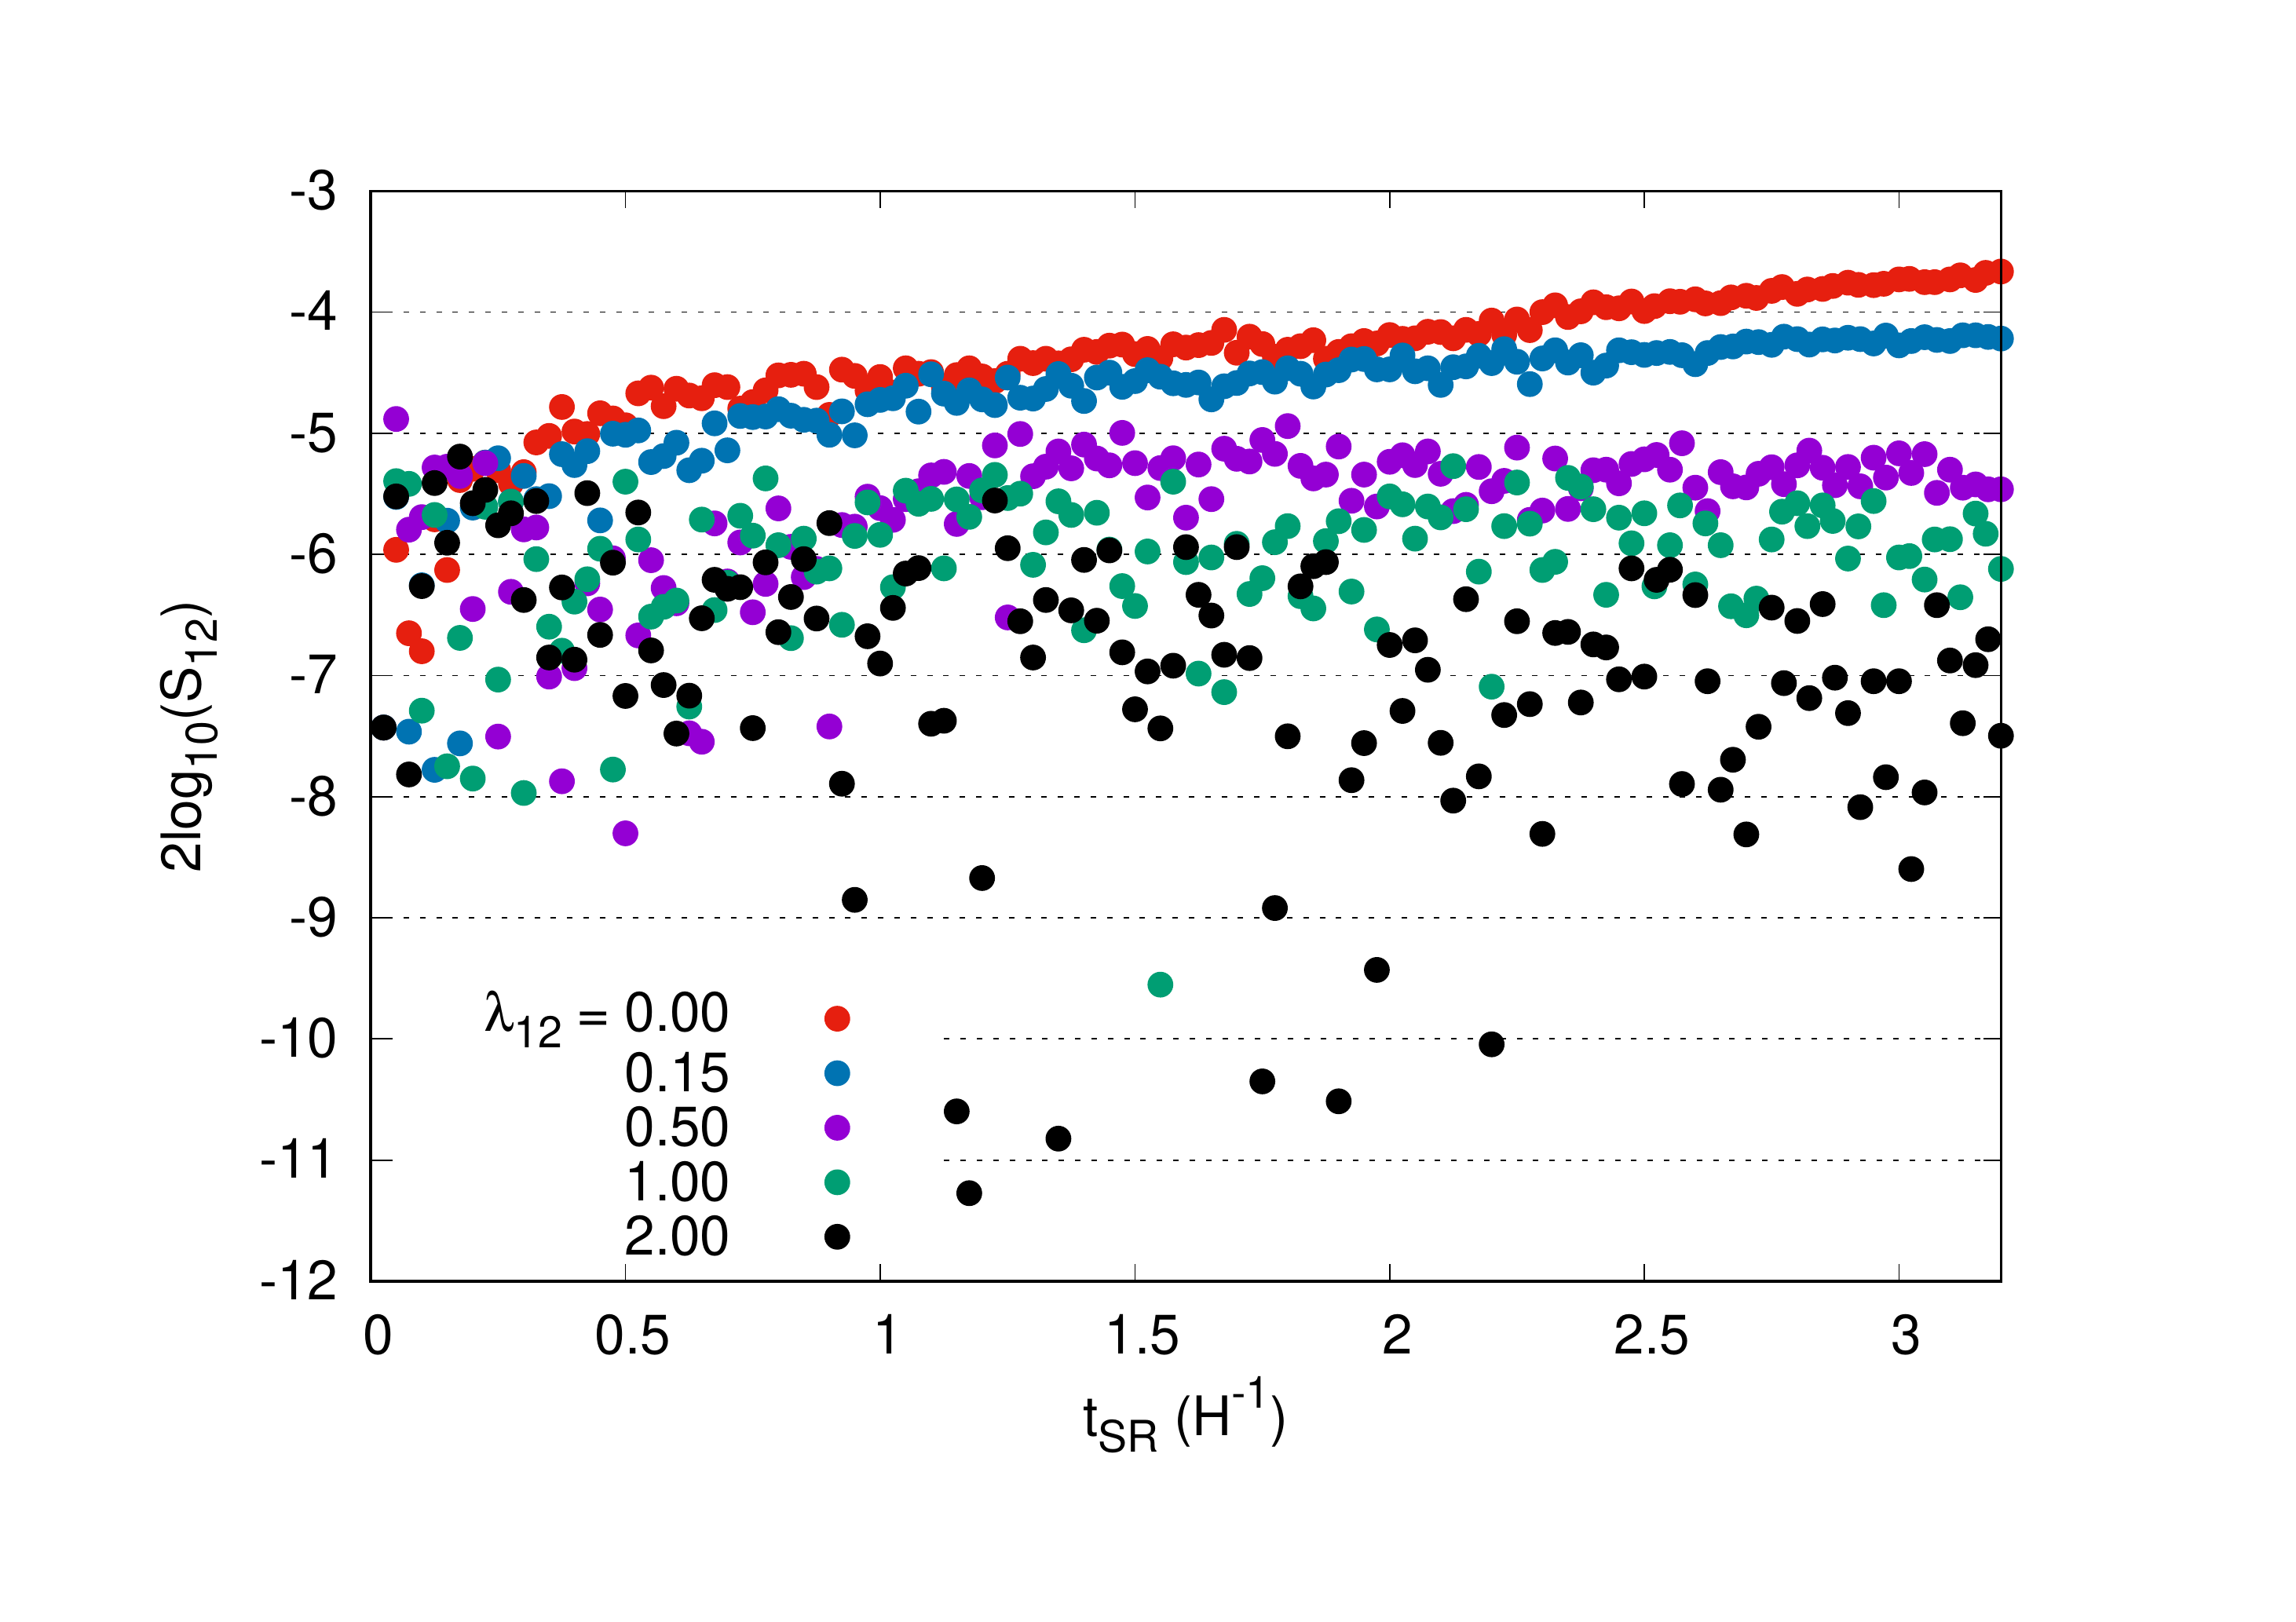}
	\caption{\label{fig:glyoxal-overlap} The effective overlap between the ground- and excited-state wave function ($|S_{12}|^2$) of glyoxal [CIPSI (NO) 5046 determinants (see Table~\ref{tab:glyoxal-SI})] plotted throughout the SR optimization for different values of $\lambda_{12}$. The sampling at a given step increases as $t_{\mathrm{SR}}$ increases.}
\end{center}
\end{figure}

% 1. Make font larger
% 2. Change 'lambda' in key to Greek symbol
% 3. The y axis label should be defined outside the plot as something simpler, then used in the image instead of the explicit form.
% 4. Add A), B), or something?
% 5. Add a line for the initial overlap for all. 3.724459205732803E-008
% 6. Change colors, don't use yellow

% should really do this on a different system, with a small expansion, quickly to see if the same thing occurs. It is weird the ground-state changes but not the excited state. Why would the GS ever increase in energy? Well, if the energy surface found sees the higher energy as the mimnima at that SR step.
