# Supplementary material for: Double excitation energies from quantum Monte Carlo using state-specific energy optimization
Source: arXiv:2207.12160 source file (2022-07-25)
Supplement: Supplementary file 15 [file glyoxal-table-SI.tex]

\begin{table*}[!htb]
\caption{Glyoxal VMC and DMC results. The optimal weights ($w_1^{\mathrm{inp}}-w_2^{\mathrm{inp}}$) in the CAS basis are 0.50$-$0.50 (< 5,000 determinants) and  0.475$-$0.525 (> 5,000 determinants). The optimal weights in the NO basis are 0.45$-$0.55.}
%\caption{Glyoxal VMC and DMC total energies (a.u.) and excitation energies (eV). The number of determinants (\#~det) and parameters (\#~parm) in each trial wave function are also presented. CIPSI expansions in the CAS basis use the optimized orbitals from a SA(2)-CASSCF(14,12) calculation with irrep $\mathrm{^1A_{g}}$ ($\mathrm{C_{2h}}$) using BFD pseudopotentials with the corresponding aug-cc-pVDZ basis set. The optimal weights ($w_1^{\mathrm{inp}}-w_2^{\mathrm{inp}}$) in the CAS basis are 0.50$-$0.50. Results for weights of 0.475$-$0.525 are also provided. The optimal weights in the NO basis are 0.45$-$0.55.}
\resizebox{\columnwidth}{!}{
\begin{tabular}{lrrllllll}
\hline
 & & & \multicolumn{3}{c}{VMC} & \multicolumn{3}{c}{DMC} \\ 
\cline{4-6}
\cline{7-9}
\multicolumn{1}{c}{WF} & \multicolumn{1}{c}{\# det} & \multicolumn{1}{c}{\# parm} & \multicolumn{1}{c}{$E\left(1 ^1\mathrm{A_g}\right)$} & \multicolumn{1}{c}{$E\left(2 ^1\mathrm{A_g}\right)$} & \multicolumn{1}{c}{$\Delta E$} & \multicolumn{1}{c}{$E\left(1 ^1\mathrm{A_g}\right)$} & \multicolumn{1}{c}{$E\left(2 ^1\mathrm{A_g}\right)$} & \multicolumn{1}{c}{$\Delta E$} \\
\hline
%\multicolumn{9}{l}{\bf State-average} \\
%\multicolumn{9}{c}{BFD/aug-cc-pVDZ} \\[1ex]
%\color{red} CAS(8,6)  &   61  &   441 & -44.5545(2) & -44.3430(2) & 5.755(7) & -44.6392(1) & -44.4295(1) & 5.705(5) \\
%            &       &       &             &             &          & -44.6410(2) & -44.4314(2) & 5.704(6) \\ % tau=0.05
%CAS(12,8) (disregarding)   &  208  &   507 & -44.5563(2) & -44.3482(2) & 5.662(7) &             &             &          \\
%            &       &       &             &             &          & -44.6422(2) & -44.4341(2) & 5.663(6) \\ % tau=0.05
%CIPSI-5,5    & 1632  &\\[1ex]
%\multicolumn{9}{l}{\bf State-specific} \\
%\multicolumn{9}{c}{BFD/aug-cc-pVDZ} \\[1ex]
%CAS(8,6) conv not acc  &    61 &  441 & -44.5600(1) & -44.3460(1) & 5.823(5)  & -44.6419(1)   & -44.4307(1)   & 5.745(5) \\
CAS(8,6)                &    61 &  441 & -44.5603(2) & -44.3473(2) & 5.79(1)   & -44.6428(3)   & -44.4315(3)   & 5.75(1) \\[.5ex]
%                       &       &      &               &             &         & -44.64446(16) & -44.43247(16) & 5.768(6) \\ % tau=0.05
%CAS(12,8) disregarding &   208 &  506 & -44.5611(2) & -44.3510(2) & 5.717(8)  & -44.6425(1)   & -44.4339(1)   & 5.676(4) \\[.5ex]
%CIPSI-5,5  (ok, inej)  &   358 &  816 & -44.5727(1) & -44.3627(1) & 5.716(4)  & -44.6437(1)   & -44.4367(1)   & 5.633(5) \\
\hline
\multicolumn{9}{l}{CIPSI (CAS)}\\
0.50$-$0.50                   &   358 &  816 & -44.5729(2) & -44.3633(2) & 5.70(1)   & -44.6437(2)   & -44.4369(2)   & 5.63(1) \\
%(ok, inej)             &  1632 & 2683 & -44.5936(1) & -44.3824(1) & 5.746(3)  & -44.6507(1)   & -44.4431(1)   & 5.648(4) \\
                        &  1632 & 2683 & -44.5950(2) & -44.3832(2) & 5.76(1)   & -44.6514(3)   & -44.4434(3)   & 5.66(1) \\
%needs a bit lower error&  3446 & 3903 & -44.6065(1) & -44.3953(1) & 5.749(3)  & -44.6564(1)   & -44.4484(1)   & 5.659(4) \\
                        &  3446 & 3903 & -44.6075(2) & -44.3965(2) & 5.74(1)   & -44.6565(2)   & -44.4494(2)   & 5.64(1) \\
%                       & 10342 & 7248 & -44.6253(1) & -44.4116(1) & 5.814(3)  & -44.6658(1)   & -44.4561(1)   & 5.708(4) \\[.5ex]
%                       & 10342 & 7248 & -44.6270(1) & -44.4127(1) & 5.833(3)  & (1) & (1) & (4) \\[.5ex]
                        & 10342 & 7248 & -44.6273(2) & -44.4124(2) & 5.85(1)   & -44.6663(2)   & -44.4567(2)   & 5.70(1) \\[.5ex]
%CIPSI-45,55 (ok, inej) & 10682 & 7423 & -44.6259(1) & -44.4129(1) & 5.795(3)  & -44.6660(1)   & -44.4569(1)   & 5.688(4) \\[1ex]
%CIPSI-45,55             & 10682 & 7423 & -44.6262(2) & -44.4141(2) & 5.77(1)   & -44.6665(2)   & -44.4574(2)   & 5.69(1) \\[1ex]
%CIPSI-4,6 CID-fNO       &  2336 & 5381 & -44.6008(1) & -44.3848(1) & 5.878(3)  & -44.6530(1)   & -44.4438(1)   & 5.695(5) \\
0.475$-$0.525           & 10660 & 7374 & -44.6288(2) & -44.4160(2) & 5.79(1) & -44.6675(2) & -44.4585(2) & 5.69(1) \\[.5ex]
\hline
\multicolumn{9}{l}{CIPSI (NO)}\\
0.45$-$0.55   &  3749 & 2908 & -44.6072(2) & -44.3957(2) & 5.76(1)   & -44.6564(2)   & -44.4482(2)   & 5.67(1) \\
                        &  5046 & 3498 & -44.6127(2) & -44.4004(2) & 5.78(1)   & -44.6600(2)   & -44.4509(2)   & 5.69(1) \\
                        &  7040 & 4500 & -44.6150(2) & -44.4048(2) & 5.72(1)   & -44.6613(2)   & -44.4534(2)   & 5.66(1) \\
                        &  8642 & 5433 & -44.6181(2) & -44.4098(2) & 5.67(1)   & -44.6632(2)   & -44.4559(2)   & 5.64(1) \\
                        & 10010 & 6188 & -44.6205(2) & -44.4114(2) & 5.69(1)   & -44.6635(2)   & -44.4567(2)   & 5.63(1) \\
                        & 12132 & 6269 & -44.6237(2) & -44.4145(2) & 5.70(1)   & -44.6654(2)   & -44.4576(2)   & 5.66(1) \\
                        & 15349 & 8577 & -44.6276(2) & -44.4180(2) & 5.70(1)   & -44.6670(2)   & -44.4600(2)   & 5.63(1) \\
%CIPSI-5,5 HF50-NO      & 10483 & 6354 & -44.617(5)  & -44.403(5)  & 5.8(2)    & (1) & (1) & (5) \\
%\multicolumn{9}{c}{BFD/aug-cc-pVTZ} \\[1ex]
%\color{red} CIPSI-55,45  &   329 &  1371 & -44.5783(1) & -44.3654(1) & 5.794(3) & -44.6453(1) & -44.4366(1) & 5.679(5) \\
%             &  1514 &  5564 & -44.5938(1) & -44.3824(1) & 5.752(3) & (1) & (1) & (4) \\
%             &  3169 &  9474 & -44.6091(1) & -44.3921(1) & 5.906(3) & (1) & (1) & (5) \\
%             & 10914 & 18303 & -44.6282(1) & -44.4132(1) & 5.850(3) & (1) & (1) & (5) \\
\hline
\multicolumn{8}{l}{TBE$^a$}         &  \multicolumn{1}{l}{5.61} \\
%\multicolumn{8}{l}{exFCI/AVDZ}            &  \multicolumn{1}{l}{5.48(0)} \\
%\multicolumn{8}{l}{CIPSI-Anthony}         &  \multicolumn{1}{l}{5.56(11)} \\
\multicolumn{8}{l}{CC3/AVQZ$^b$}            &  \multicolumn{1}{l}{6.76} \\
%\multicolumn{8}{l}{PP-CC3 (\%T$_1$)/BFD-AVDZ$^b$} &  \multicolumn{1}{l}{6.75 (0.84\%)} \\
%\multicolumn{8}{l}{FC-CC3 (\%T$_1$)/AVDZ$^b$}    &  \multicolumn{1}{l}{6.71 (0.71\%)} \\
%\multicolumn{8}{l}{AE-CC3 (\%T$_1$)/AVDZ$^b$}    &  \multicolumn{1}{l}{6.70 (0.69\%)} \\
%\multicolumn{8}{l}{PP-CC3 (\%T$_1$)/BFD-AVTZ$^b$} &  \multicolumn{1}{l}{6.81 (0.64\%)} \\
%\multicolumn{8}{l}{FC-CC3 (\%T$_1$)/AVTZ$^b$}    &  \multicolumn{1}{l}{6.76 (0.54\%)} \\
%\multicolumn{8}{l}{AE-CC3 (\%T$_1$)/AVTZ$^b$}    &  \multicolumn{1}{l}{6.75 (0.51\%)} \\
%\multicolumn{8}{l}{FC-CC3 (\%T$_1$)/AVQZ} &  \multicolumn{1}{l}{6.76 (1\%)} \\
\multicolumn{8}{l}{CC4/6-31+G*$^c$}           &  \multicolumn{1}{l}{5.699} \\
\multicolumn{8}{l}{CC4/AVDZ$^c$}              &  \multicolumn{1}{l}{5.593} \\
\multicolumn{8}{l}{CCSDTQ/6-31+G*$^c$}        &  \multicolumn{1}{l}{5.670} \\
%\multicolumn{8}{l}{CASPT2(8,6)/AVDZ}      &  \multicolumn{1}{l}{5.55} \\
%\multicolumn{8}{l}{CASPT2(8,6)/AVQZ}      &  \multicolumn{1}{l}{5.52} \\
%\multicolumn{8}{l}{CASPT2(14,12)/AVDZ}    &  \multicolumn{1}{l}{5.47} \\
\multicolumn{8}{l}{exFCI/AVDZ}    &  \multicolumn{1}{l}{5.56(11)} \\
\multicolumn{8}{l}{SAC-CI/AVDZ$^d$}    &  \multicolumn{1}{l}{5.66} \\
\multicolumn{8}{l}{CASPT2(14,12)/AVQZ$^b$}    &  \multicolumn{1}{l}{5.43} \\
%\multicolumn{8}{l}{PC-NEVPT2(14,12)/AVDZ} &  \multicolumn{1}{l}{5.56} \\
\multicolumn{8}{l}{PC-NEVPT2(14,12)/AVQZ$^b$} &  \multicolumn{1}{l}{5.52} \\
%\multicolumn{8}{l}{SC-NEVPT2(14,12)/AVDZ} &  \multicolumn{1}{l}{5.58} \\
%\multicolumn{8}{l}{SC-NEVPT2(14,12)/AVQZ} &  \multicolumn{1}{l}{5.55} \\
\hline
\multicolumn{8}{l}{$^a$This value is `safe', as defined in Ref.~\citenum{questdb}. exFCI/AVDZ + ( CCSDT/AVTZ - CCSDT/AVDZ ) } \\
\multicolumn{8}{l}{$^b$Ref.~\citenum{loos2019}.} \\
\multicolumn{8}{l}{$^c$Ref.~\citenum{newcc4}.} \\
\multicolumn{8}{l}{$^d$Ref.~\citenum{SACCI}. See reference for basis set details.} \\
\end{tabular}
}
\label{tab:glyoxal-SI}
\end{table*}
