# Supplementary material for: Double excitation energies from quantum Monte Carlo using state-specific energy optimization
Source: arXiv:2207.12160 source file (2022-07-25)
Supplement: Supplementary file 20 [file nitroxyl-table-SI.tex]

\begin{table*}[!htb]
\caption{Nitroxyl VMC and DMC results. The optimal weights ($w_1^{\mathrm{inp}}-w_2^{\mathrm{inp}}$) in the CAS basis are 0.525$-$0.475. Results for weights of 0.50$-$0.50 are also provided. The optimal weights in the NO basis are 0.50$-$0.50.}
%\caption{Nitroxyl VMC and DMC total energies (a.u.) and excitation energies (eV). The number of determinants (\#~det) and parameters (\#~parm) in each trial wave function are also presented. CIPSI expansions in the CAS basis use the optimized orbitals from a SA(2)-CASSCF(12,9) calculation with irrep $\mathrm{^1A'}$ ($\mathrm{C_s}$) using BFD pseudopotentials with the corresponding aug-cc-pVDZ basis set. The optimal weights ($w_1^{\mathrm{inp}}-w_2^{\mathrm{inp}}$) in the CAS basis are 0.525$-$0.475. Results for weights of 0.50$-$0.50 are also provided. The optimal weights in the NO basis are 0.50$-$0.50.}
\resizebox{\columnwidth}{!}{
\begin{tabular}{lrrllllll}
\hline
 & & & \multicolumn{3}{c}{VMC} & \multicolumn{3}{c}{DMC} \\
\cline{4-6}
\cline{7-9}
\multicolumn{1}{c}{WF} & \multicolumn{1}{c}{\# det} & \multicolumn{1}{c}{\# parm} & \multicolumn{1}{c}{$E\left(1 ^1\mathrm{A'}\right)$} & \multicolumn{1}{c}{$E\left(2 ^1\mathrm{A'}\right)$} & \multicolumn{1}{c}{$\Delta E$} & \multicolumn{1}{c}{$E\left(1 ^1\mathrm{A'}\right)$} & \multicolumn{1}{c}{$E\left(2 ^1\mathrm{A'}\right)$} & \multicolumn{1}{c}{$\Delta E$} \\
\hline
%\multicolumn{9}{l}{\bf State-average} \\[.5ex]
%CAS(12,9) & 3528 & 1599 &  -26.4721(1) &  -26.3099(1) & 4.413(4) & -26.5093(1) & -26.3492(1) & 4.357(4) \\
%  0.0125 & -26.5090(1) & -26.3488(1) & 4.359(5) \\
%  0.0200 & -26.5093(1) & -26.3492(1) & 4.357(4) \\
%  0.0500 & -26.5113(1) & -26.3509(1) & 4.364(4) \\
%  0.0250 & -26.5096(1) & -26.3495(1) & 4.358(4) \\
%\multicolumn{9}{l}{\bf State-specific} \\[.5ex]
CAS(2,2)   &    2   &  231 &  -26.4462(3) &  -26.2764(3) &  4.61(1) & -26.4990(2) & -26.3321(2) & 4.54(1) \\
CAS(12,9)  & 3528   & 1598 &  -26.4762(2) &  -26.3134(2) & 4.43(1) & -26.5114(2) & -26.3510(2) & 4.36(1) \\[.5ex]
\hline
\multicolumn{9}{l}{CIPSI (CAS)} \\
0.50$-$0.50  &  363   &  965 & -26.4876(2) & -26.3236(2) & 4.46(1) & -26.5161(2) & -26.3547(2) & 4.39(1) \\
           &  1627  & 2150 & -26.5013(2) & -26.3426(2) & 4.32(1) & -26.5228(2) & -26.3643(2) & 4.31(1) \\
           &  3447  & 2986 & -26.5061(2) & -26.3469(2) & 4.33(1) & -26.5248(2) & -26.3661(2) & 4.32(1) \\
           &  10660 & 5826 & -26.5106(2) & -26.3506(2) & 4.35(1) & -26.5267(2) & -26.3675(2) & 4.33(1) \\[.5ex]
0.525$-$0.475&    322 &  909 & -26.4891(2) & -26.3271(2) & 4.41(1) & -26.5155(2) & -26.3565(2) & 4.33(1) \\
           &   1569 & 2126 & -26.5021(2) & -26.3423(2) & 4.35(1) & -26.5228(2) & -26.3644(2) & 4.31(1) \\
           &   3751 & 3135 & -26.5088(2) & -26.3481(2) & 4.37(1) & -26.5260(2) & -26.3667(2) & 4.33(1) \\
           &   7464 & 4618 & -26.5111(2) & -26.3511(2) & 4.35(1) & -26.5273(2) & -26.3682(2) & 4.33(1) \\
           &  10516 & 5772 & -26.5119(2) & -26.3517(2) & 4.36(1) & -26.5275(2) & -26.3680(2) & 4.34(1) \\[.5ex]
\hline
\multicolumn{9}{l}{CIPSI (NO)} \\
0.50$-$0.50  &    321 &  850 & -26.4917(2) & -26.3322(2) & 4.34(1) & -26.5164(2) &
           -26.3583(2) & 4.30(1) \\
           &   1573 & 1446 & -26.5001(2) & -26.3415(2) & 4.31(1) & -26.5220(2) & -26.3636(2) & 4.31(1) \\
           &   2900 & 2002 & -26.5040(2) & -26.3447(2) & 4.34(1) & -26.5240(2) & -26.3652(2) & 4.32(1) \\
           &   7171 & 4124 & -26.5102(2) & -26.3498(2) & 4.36(1) & -26.5267(2) & -26.3677(2) & 4.33(1) \\
           &  10690 & 5712 & -26.5113(2) & -26.3519(2) & 4.34(1) & -26.5273(2) & -26.3686(2) & 4.32(1) \\
\hline
\multicolumn{8}{l}{TBE$^a$}       & \multicolumn{1}{l}{4.33} \\
\multicolumn{8}{l}{CC3/AVQZ$^b$} & \multicolumn{1}{l}{5.23} \\
\multicolumn{8}{l}{CC4/AVDZ$^c$}               & \multicolumn{1}{l}{4.454} \\
\multicolumn{8}{l}{CC4/AVTZ$^c$}               & \multicolumn{1}{l}{4.380} \\
\multicolumn{8}{l}{CCSDT/AVDZ$^b$}         & \multicolumn{1}{l}{4.756} \\
\multicolumn{8}{l}{CCSDTQ/AVDZ$^b$}        & \multicolumn{1}{l}{4.424} \\
\multicolumn{8}{l}{CCSDTQ/AVTZ$^c$}            & \multicolumn{1}{l}{4.364} \\
%\multicolumn{8}{l}{FCI/AVDZ$^b$}           & \multicolumn{1}{l}{4.397(1)} \\
%\multicolumn{8}{l}{exFCI/AVDZ$^d$}         & \multicolumn{1}{l}{4.40(1)} \\
\multicolumn{8}{l}{exFCI/AVQZ$^d$}         & \multicolumn{1}{l}{4.32(0)} \\
%\multicolumn{8}{l}{CASPT2(12,9)/AVDZ$^d$}  & \multicolumn{1}{l}{4.46} \\
\multicolumn{8}{l}{CASPT2(12,9)/AVQZ$^d$}  & \multicolumn{1}{l}{4.34} \\
%\multicolumn{8}{l}{PC-NEVPT2(12,9)/AVDZ$^d$} & \multicolumn{1}{l}{4.46} \\
\multicolumn{8}{l}{PC-NEVPT2(12,9)/AVQZ$^d$} & \multicolumn{1}{l}{4.35} \\
\hline
\multicolumn{8}{l}{$^a$Value is `safe', as defined in Ref.~\citenum{questdb}. FCI/AVTZ}\\
\multicolumn{8}{l}{$^b$Ref.~\citenum{loos2021}.}\\
\multicolumn{8}{l}{$^c$Ref.~\citenum{newcc4}.}\\
\multicolumn{8}{l}{$^d$Ref.~\citenum{loos2019}.}\\
\end{tabular}
}
\label{tab:nitroxyl-SI}
\end{table*}
