# Supplementary material for: Double excitation energies from quantum Monte Carlo using state-specific energy optimization
Source: arXiv:2207.12160 source file (2022-07-25)
Supplement: Supplementary file 21 [file si-title.tex]

\title{Supporting Information: Accurate double excitation energies using penalty-based quantum Monte Carlo optimization}
