# Supplementary material for: Double excitation energies from quantum Monte Carlo using state-specific energy optimization
Source: arXiv:2207.12160 source file (2022-07-25)
Supplement: Supplementary file 23 [file tetrazine-cipsi-fig.tex]

\begin{figure}[htb]
\begin{center}
\includegraphics[scale=0.363]{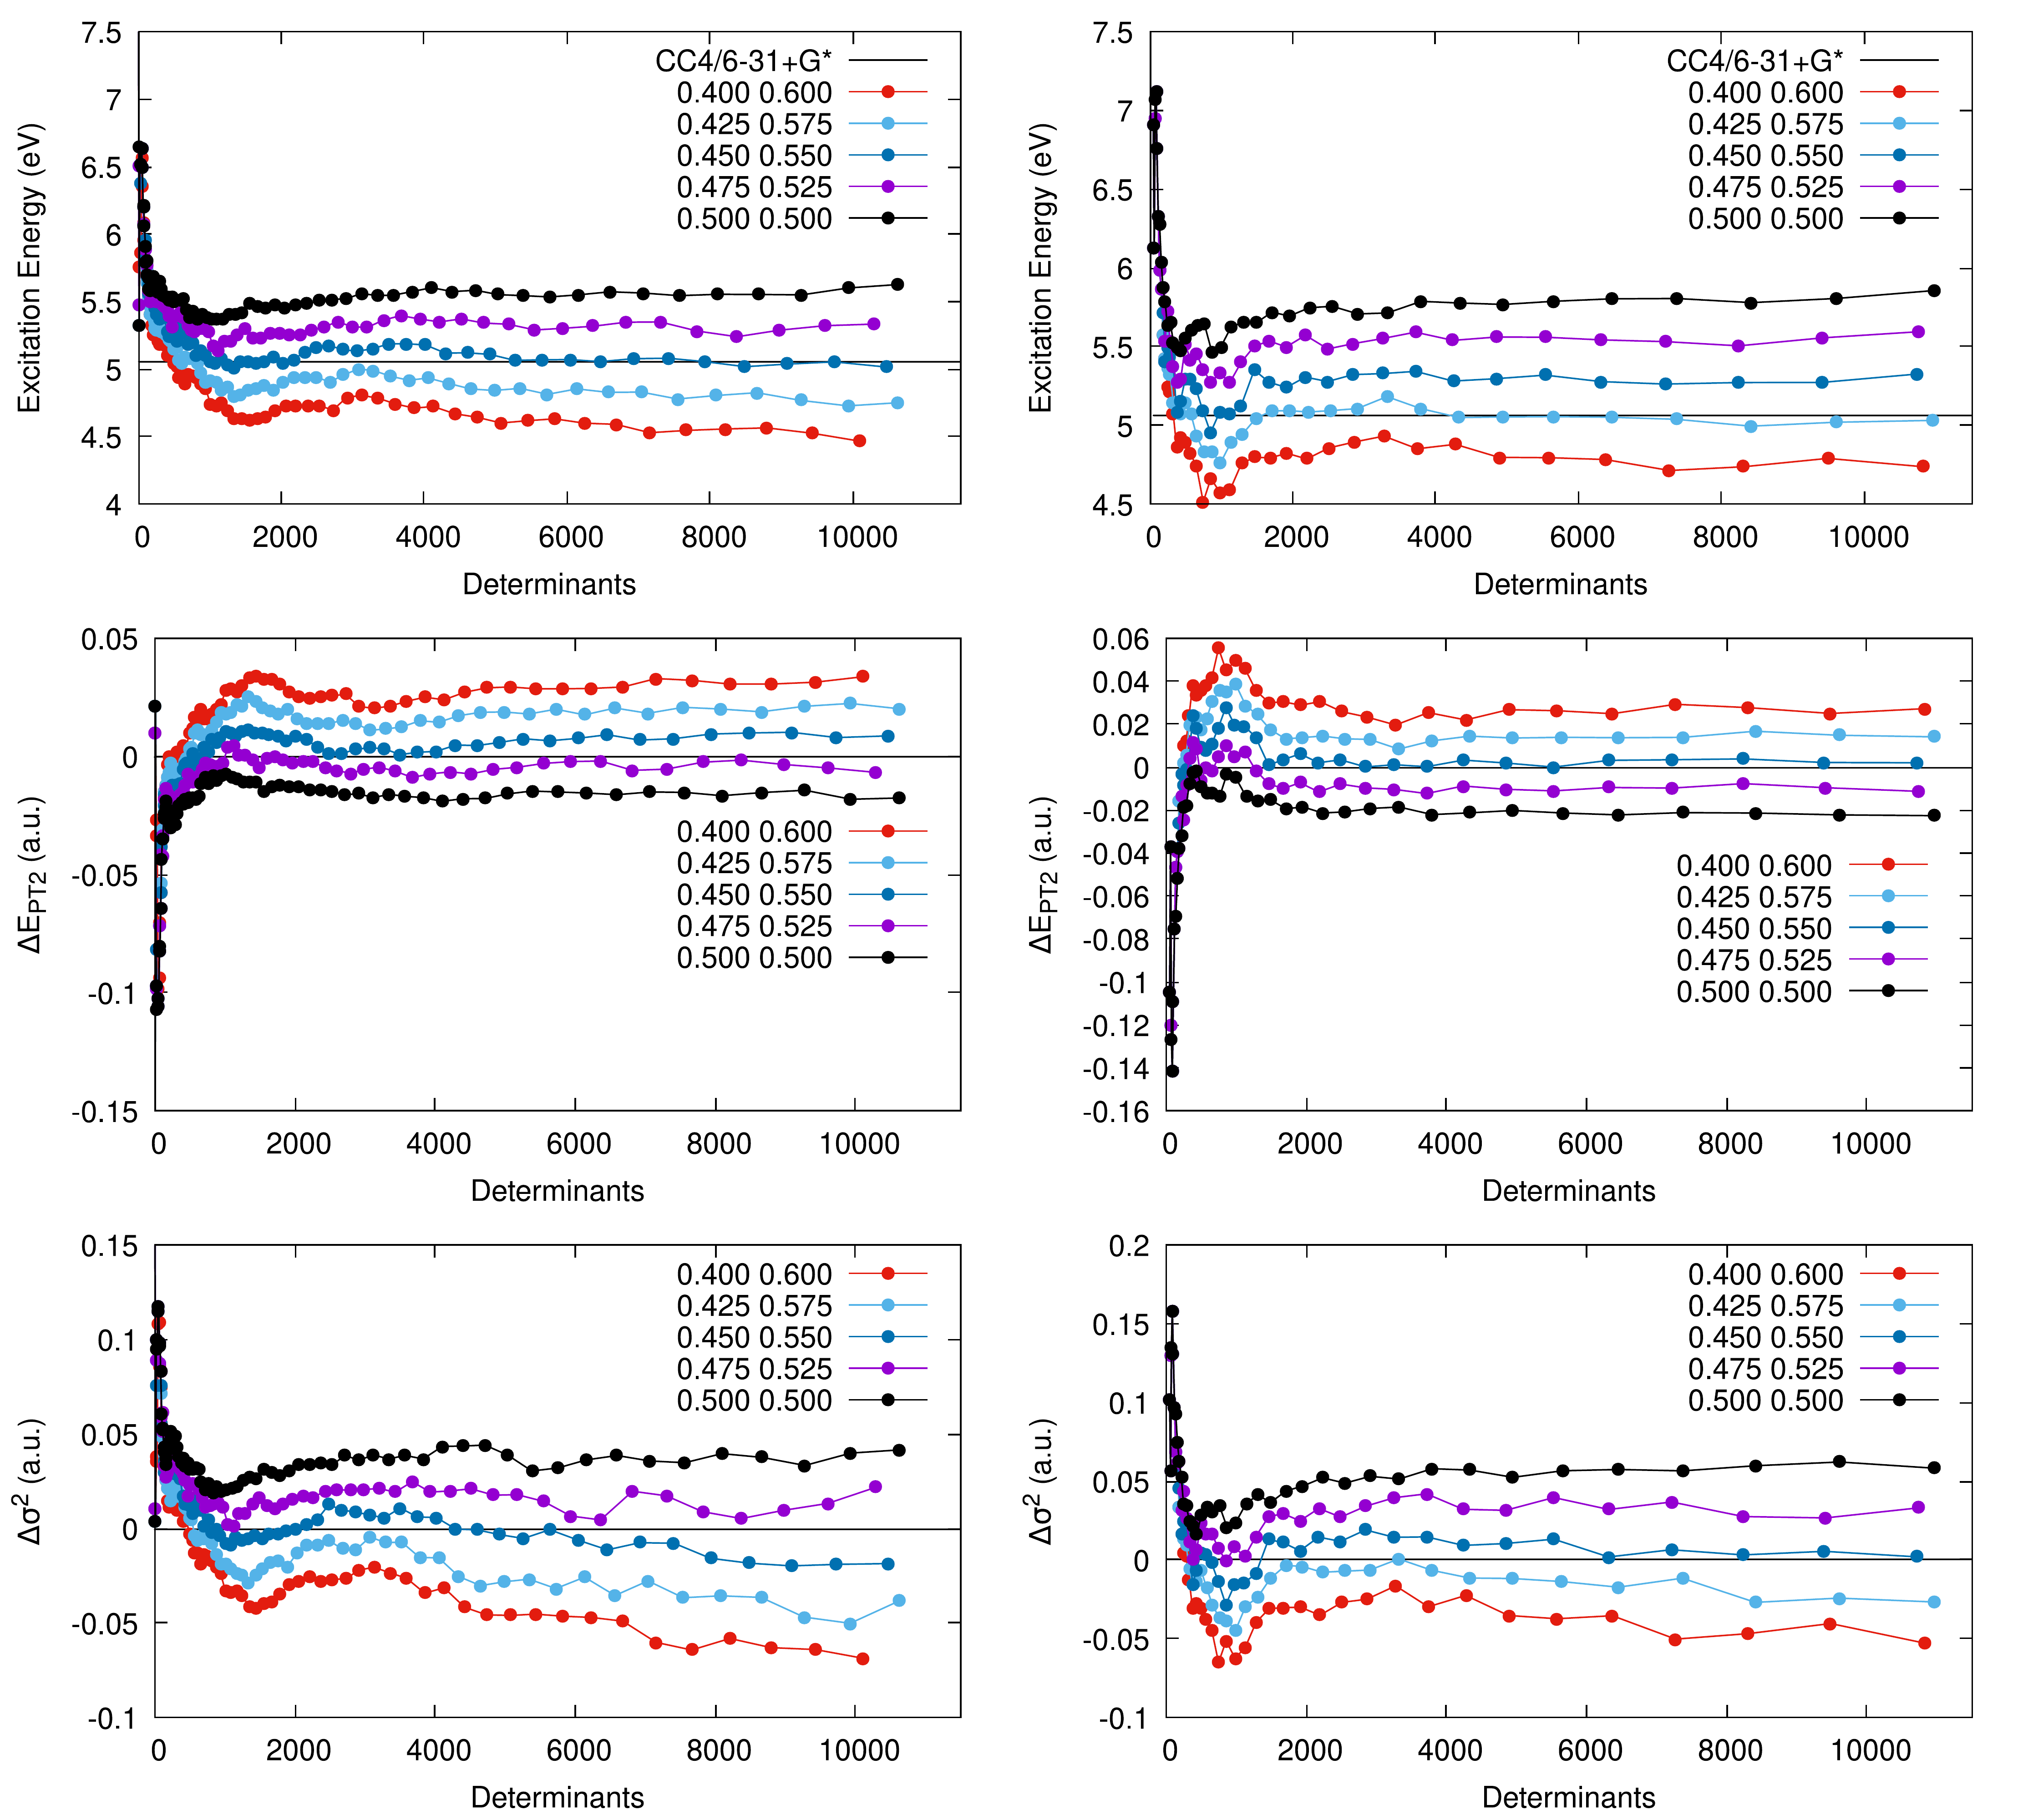}
\caption{\label{fig:tetrazine-cipsi} Tetrazine CIPSI energies, PT2 energies, and variances in the CAS (left) and NO (right) basis, using different input weights ($w_1^{\mathrm{inp}}$ $w_2^{\mathrm{inp}}$).}
\end{center}
\end{figure}
