# Supplementary material for: Double excitation energies from quantum Monte Carlo using state-specific energy optimization
Source: arXiv:2207.12160 source file (2022-07-25)
Supplement: Supplementary file 25 [file tetrazine-table-SI.tex]

\begin{table*}[!htb]
\caption{Tetrazine VMC and DMC results. The optimal weights ($w_1^{\mathrm{inp}}-w_2^{\mathrm{inp}}$) in the  CAS and NO basis are 0.45$-$0.55.}
%\caption{Tetrazine VMC and DMC total energies (a.u.) and excitation energies (eV). The number of determinants (\#~det) and parameters (\#~parm) in each trial wave function are also presented. CIPSI expansions in the CAS basis use the optimized orbitals from a SA(2)-CASSCF(14,10) calculation with irrep $\mathrm{^1A_{1g}}$ ($\mathrm{D_{2h}}$) using BFD pseudopotentials with the corresponding aug-cc-pVDZ basis set. The optimal weights ($w_1^{\mathrm{inp}}-w_2^{\mathrm{inp}}$) in the  CAS and NO basis are 0.45$-$0.55.}
\resizebox{\columnwidth}{!}{
\begin{tabular}{lrrllllll}
\hline
 & & & \multicolumn{3}{c}{VMC} & \multicolumn{3}{c}{DMC} \\ 
\cline{4-6}
\cline{7-9}
\multicolumn{1}{c}{WF} & \multicolumn{1}{c}{\# det} & \multicolumn{1}{c}{\# parm} & \multicolumn{1}{c}{$E\left(1 ^1\mathrm{A_{1g}}\right)$} & \multicolumn{1}{c}{$E\left(2 ^1\mathrm{A_{1g}}\right)$} & \multicolumn{1}{c}{$\Delta E$} & \multicolumn{1}{c}{$E\left(1 ^1\mathrm{A_{1g}}\right)$} & \multicolumn{1}{c}{$E\left(2 ^1\mathrm{A_{1g}}\right)$} & \multicolumn{1}{c}{$\Delta E$} \\
\hline
%\multicolumn{9}{l}{\bf State-average} \\
%\multicolumn{9}{c}{BFD/aug-cc-pVDZ} \\[1ex]
%CAS(4,4)    &    6 &  400 & -52.1496(6)  & -51.9507(6) & 5.41(2)  & -52.2647(2)   & -52.0744(2)   & 5.179(7)$^a$ \\
%            &      &      & -52.1482(1)  & -51.9504(1) & 5.382(4) & -52.2641(2)   & -52.0740(2)   & 5.173(9)     \\
%CAS(8,6)    &   33 &  415 & -52.1627(7)  & -51.9550(7) & 5.65(3)  & -52.2728(2)   & -52.0769(2)   & 5.332(7)$^a$ \\
%CAS(12,8)   &  112 &  455 & -52.1643(6)  & -51.9644(6) & 5.44(2)  & -52.2738(2)   & -52.0828(2)   & 5.196(7)$^a$ \\
%CAS(14,10)  & 1824 & 1139 & -52.1732(1)  & -51.9840(1) & 5.148(5) & -52.2784(2)   & -52.0922(2)   & 5.067(7)$^a$ \\
%            &      &      &              &             &          & -52.27720(16) & -52.09097(16) & 5.068(6)     \\
%CIPSI-400  &  385 &  871 & -52.1609(1)  & -51.9785(1) & 4.965(4) & -52.2684(1)   & -52.0863(1)   & 4.955(5)     \\
%\multicolumn{9}{l}{\bf State-specific} \\
%\multicolumn{9}{c}{BFD/aug-cc-pVDZ} \\[1ex]
%CAS(4,4) bad        &     6 &  399 & -52.1496(1) & -51.9513(1) & 5.394(4) & -52.2647(2)   & -52.0732(2)   & 5.213(8) \\
CAS(4,4)             &     6 &  399 & -52.1492(2) & -51.9510(2) & 5.39(1)  & -52.2647(3)   & -52.0734(3)   & 5.21(1) \\
%CAS(8,6) ok         &    33 &  414 & -52.1645(1) & -51.9566(1) & 5.657(4) & -52.2724(2)   & -52.0761(2)   & 5.342(7) \\
CAS(8,6)             &    33 &  414 & -52.1649(2) & -51.9569(2) & 5.66(1)  & -52.2725(3)   & -52.0767(3)   & 5.33(1) \\
CAS(12,8)            &   112 &  454 & -52.1652(2) & -51.9658(2) & 5.43(1)  & -52.2740(3)   & -52.0824(3)   & 5.21(1)  \\
%CAS(14,10)          &  1824 & 1078 & -52.1778(2) & -51.9887(2) & 5.147(9) & -52.2805(1)   & -52.0941(1)   & 5.071(4) \\
CAS(14,10)           &  1824 & 1078 & -52.1772(2) & -51.9880(2) & 5.15(1)  & -52.2804(3)   & -52.0927(3)   & 5.11(1) \\[.5ex]
%CIPSI-45,55 close   &   385 &  871 & -52.1823(1) & -52.0002(1) & 4.957(4) & -52.2808(1)   & -52.0974(1)   & 4.990(6) \\
\hline
\multicolumn{9}{l}{CIPSI (CAS)} \\
0.45$-$0.55   &   385 &  871 & -52.1826(2) & -52.0008(2) & 4.95(1)  & -52.2811(3)   & -52.0985(3)   & 4.97(1) \\
%            close   &  1757 & 1608 & -52.1952(1) & -52.0200(1) & 4.766(4) & -52.2837(1)   & -52.1039(1)   & 4.890(5) \\
                     &  1757 & 1608 & -52.1966(2) & -52.0203(2) & 4.80(1)  & -52.2841(2)   & -52.1042(2)   & 4.89(1) \\
%            close   &  3718 & 2302 & -52.2124(1) & -52.0313(1) & 4.928(3) & -52.2912(1)   & -52.1088(1)   & 4.964(5) \\
                     &  3718 & 2302 & -52.2138(2) & -52.0323(2) & 4.94(1)  & -52.2918(3)   & -52.1089(3)   & 4.98(1) \\
%good, do inej       & 10470 & 6934 & -52.2314(1) & -52.0496(2) & 4.945(7) & -52.2990(1)   & (2) & (6) \\
                     & 10470 & 6934 & -52.2321(2) & -52.0504(2) & 4.94(1)  & -52.2996(2)   & -52.1171(2)   & 4.97(1) \\[.5ex]
\hline
\multicolumn{9}{l}{CIPSI (NO)} \\
0.45$-$0.55   &  3572 & 2414 & -52.2198(2) & -52.0346(2) & 5.04(1)  & -52.2935(3)   & -52.1098(3)   & 5.00(1) \\
                     &  7025 & 4141 & -52.2300(2) & -52.0451(2) & 5.03(1)  & -52.2981(3)   & -52.1148(3)   & 4.99(1) \\
                     & 10723 & 6053 & -52.2379(2) & -52.0528(2) & 5.04(1)  & -52.3015(3)   & -52.1182(3)   & 4.99(1) \\
%CIPSI-5,5  good, do inej & 10628 & 4422 & -52.2350(1) & -52.0473(1) & 5.108(3) & -52.3003(1)   & -52.1152(1)   & 5.037(5) \\
\hline
\multicolumn{8}{l}{TBE$^a$}                  &  \multicolumn{1}{l}{4.61} \\
%\multicolumn{8}{l}{CCSDT/AVDZ}               &  \multicolumn{1}{l}{5.86} \\
\multicolumn{8}{l}{CC3/6-31+G*$^b$}                 &  \multicolumn{1}{l}{6.22} \\
\multicolumn{8}{l}{CC3/AVQZ$^b$}                 &  \multicolumn{1}{l}{6.19} \\
\multicolumn{8}{l}{CC4/6-31+G*$^c$}              &  \multicolumn{1}{l}{5.06} \\
\multicolumn{8}{l}{CCSDT/AVTZ$^b$}               &  \multicolumn{1}{l}{5.96} \\
\multicolumn{8}{l}{exFCI/AVDZ}               &  \multicolumn{1}{l}{5.15(3)} \\
%\multicolumn{8}{l}{CASPT2(14,10)/AVDZ}       &  \multicolumn{1}{l}{4.79} \\
\multicolumn{8}{l}{CASPT2(14,10)/AVQZ$^b$}       &  \multicolumn{1}{l}{4.68} \\
%\multicolumn{8}{l}{PC-NEVPT2(14,10)/AVDZ}    &  \multicolumn{1}{l}{4.70} \\
\multicolumn{8}{l}{PC-NEVPT2(14,10)/AVQZ$^b$}    &  \multicolumn{1}{l}{4.60} \\
%\multicolumn{8}{l}{SC-NEVPT2(14,10)/AVDZ}    &  \multicolumn{1}{l}{4.78} \\
%\multicolumn{8}{l}{SC-NEVPT2(14,10)/AVQZ}    &  \multicolumn{1}{l}{4.68} \\
\hline
\multicolumn{8}{l}{$^a$This value is `unsafe', as defined in Ref~\citenum{questdb}. NEVTPT2/AVTZ} \\
\multicolumn{8}{l}{$^b$Ref.~\citenum{loos2019}.} \\
\multicolumn{8}{l}{$^c$Ref.~\citenum{newcc4}.} \\
\end{tabular}
}
\label{tab:tetrazine}
\end{table*}
